# Supplementary material for: Microlocal Theory of Legendrian Links and Cluster Algebras
Source: arXiv:2204.13244 source file (2023-12-28)
Supplement: Supplementary file 1 [file appendix.tex]

\setcounter{section}{0}

\section{Appendix: Quasi-Cluster Structures}

This appendix contains the necessary definitions regarding quasi-cluster structures and their associated objects, as needed for the purposes of this article. See also C.~Fraser's \cite{Fraser16_Quasi} and M.~Sherman-Bennett's \cite[Section 4.3]{ShermanBennett21_Thesis}.

Let us consider a lattice $N$ of finite rank, a saturated sublattice $N^\uf\subset N$, and a $\mathbb{Z}$-valued skew-symmetric form $\{\cdot, \cdot\}$ on the lattice $N$. The triple $(N,N^{uf},\{\cdot,\cdot\})$ is considered as input data, and it is fixed throughout. By definition, we set $M:=N^*$ and define the linear map 
\begin{align*}
    p^*:N^\uf&\longrightarrow M \\
    n&\longmapsto \{n,-\}.
\end{align*}
For instance, in the present article we use $N=H_1(L,T)$, for $L$ a Lagrangian filling and $T\sse\dd L$ a set of marked point at the boundary, $\{\cdot,\cdot\}$ the intersection form, and $N^{uf}$ the sub-lattice spanned by an $\L$-compressing system.

\begin{definition} Consider a triple $(N,N^\uf,\{\cdot,\cdot\})$ as above. A basis $\{e_i\}$ of $N^\uf$ is said to be a \emph{seed} $\mathbf{s}$ associated to $(N,N^\uf,\{\cdot,\cdot\})$.
\end{definition}

\begin{definition}
Given a seed $\mathbf{s}$ and an element $e_k\in \mathbf{s}$, the seed $\mathbf{s}':=\mu_{e_k}\mathbf{s}$ which consists of vectors
\[
e'_i=\left\{\begin{array}{ll}
    -e_k & \text{if $i=k$}, \\
    e_i+\{e_i,e_k\}_+e_k & \text{if $i\neq k$},
\end{array}\right.
\]
where $\{e_i,e_k\}_+:=\max\left(\{e_i,e_k\},0\right)$, is said to be obtained by a {\it mutation} of the seed $\mathbf{s}$ at the element $e_k$. Finally, two seeds of the same given fixed data are said to be \emph{mutation equivalent} if they can be obtained from one another via a sequence of mutations, and we denote the family of seeds that are mutation equivalent to $\mathbf{s}$ by $|\mathbf{s}|$.
\end{definition}

Consider a mutation equivalence family of seeds $|\mathbf{s}_0|$. For each seed $\mathbf{s}\in |\mathbf{s}_0|$, we consider the two algebraic tori
\[
\mathcal{A}_\mathbf{s}:=\Hom(M,\mathbb{C}^\times) \quad \text{and} \quad \mathcal{X}_\mathbf{s}:=\Hom(N,\mathbb{C}^\times).
\]

\noindent which are referred to as the \emph{seed tori} associated to $\mathbf{s}$; the former is said to be of type $A$ and the latter of type $X$. By construction. $M$ and $N$ are the character lattices of $\mathcal{A}_\mathbf{s}$ and $\mathcal{X}_\mathbf{s}$ respectively, and elements of $M$ and $N$ respectively define Laurent monomial functions on $\mathcal{A}_\mathbf{s}$ and $\mathcal{X}_\mathbf{s}$. We adopt the notation of writing these functions as $A^m$ and $X^n$ for $m\in M$ and $n\in N$. In particular, multiplication of these Laurent monomial functions corresponds to addition of elements in the corresponding lattices.

Given any two seeds $\mathbf{s}=\{e_i\}$ and $\mathbf{s}'=\mu_{e_k}\mathbf{s}$  which differ by exactly one mutation, we define the two birational maps
\begin{align*}
    \mu_{e_k}:\mathcal{A}_\mathbf{s}&\dashrightarrow \mathcal{A}_{\mathbf{s}'} & \mu_{e_k}:\mathcal{X}_\mathbf{s}& \dashrightarrow \mathcal{X}_{\mathbf{s}'}\\
    \mu_{e_k}^*(A^m)&:=A^m\left(1+A^{p^*\{e_k\}}\right)^{-\langle m,e_k\rangle} & \mu_{e_k}^*(X^n)&:=X^n\left(1+X^{e_k}\right)^{-\{n,e_k\}}.
\end{align*}

By definition, the \emph{quasi-cluster varieties} $\mathcal{A}$ and $\mathcal{X}$ are the algebraic spaces obtained by gluing the (algebraic) seed tori, of the respective types $A$ and $X$, via the birational maps $\mu_{e_k}$ as above, for every pair of mutation adjacent seeds.

\begin{remark} Intuitively, the {\it quasi} in {\it quasi}-cluster allows for a controlled ambiguity coming from the frozen variables: one allows certain rescalings of the cluster variables by Laurent monomials in frozen variables. (Scaling preserving exchange ratios.) It is possible to make additional choices so that a {\it quasi}-cluster variety becomes a cluster variety. Namely, in order to obtain a seed in the theory of cluster algebras (without the {\it quasi}), we need to extend our seed $\{e_i\}$, which was a basis for $N^{uf}$ to a basis of the entire lattice $N$; in turn this yields a dual basis $\{f_i\}$ of $M$. The mutation of the dual basis is given by
\[
f'_i=\left\{\begin{array}{ll}
    -f_k+\sum_j\{e_k,-e_j\}_+f_j & \text{if $i=k$}, \\
    f_i & \text{if $i\neq k$}. 
\end{array}\right.
\]

For simplicity, let us denote $A^{f_i}$ by $A_i$ and $A^{f'_i}$ by $A'_i$. Then the first mutation map becomes
\begin{align*}
    \mu_{e_k}^*(A'_k)=&A_k^{-1}\left(\prod_{j:\{e_k,-e_j\}>0}A_j^{\{e_k,-e_j\}}\right)\left(1+\prod_jA_j^{\{e_k,e_j\}}\right)^{-\langle -f_k+\sum_j\{e_k,-e_j\}_+f_j,e_k\rangle}\\
    =&A_k^{-1}\left(\prod_{j:\{e_k,e_j\}<0}A_j^{-\{e_k,e_j\}}+\prod_{j:\{e_k,e_j\}>0}A_j^{\{e_k,e_j\}}\right),
\end{align*}
and for $i\neq k$,
\[
\mu_{e_k}^*(A'_i)=A_i\left(1+\prod_jA_j^{\{e_k,e_j\}}\right)^{-\langle f_j,e_k\rangle}=A_i,
\]
which are precisely the classical cluster $\mathcal{A}$-mutation formulas. For the cluster $\mathcal{X}$-mutations, just note that 
\[
\mu_{e_k}^*(X'_k)=X_k^{-1}(1+X_k)^{-\{e_k,e_k\}}=X_k^{-1}
\]
and for $i\neq k$,
\[
\mu_{e_k}^*(X'_i)=X_iX_k^{\{e_i,e_k\}_+}\left(1+X_k\right)^{-\{e_i,e_k\}},
\]
which are the classical cluster $\mathcal{X}$-mutation formulas.
\end{remark}

Consider the lattice $M^\fr:=(N^\uf)^\perp$, which is the saturated sublattice of $M$ corresponding to frozen cluster $\mathcal{A}$-variables. In particular, $M^\fr$ defines a frozen subtorus $\mathcal{A}^\fr\subset \mathcal{A}_\mathbf{s}$ for each seed $\mathbf{s}$, and these frozen subtori can be (and are) glued via the identity map under mutations. Since $M^\fr$ is saturated, the quotient $M/M^\fr$ is also a lattice and any seed $\mathbf{s}=\{e_i\}$ gives rise to a dual basis $\{\overline{f}_i\}$ of $M/M^\fr$. Let us choose a lift $f_i\in M$ for each $\overline{f}_i$. The subset
\[
M_+:=M^\fr+\sum\mathbb{Z}_{\geq 0}f_i
\]
then defines a monoid of global functions on $\mathcal{A}$, which we refer to as the monoid of \emph{cluster monomials} associated with the seed $\mathbf{s}$.

Finally, {\it quasi}-cluster transformations arise as follows. Suppose $\mathbf{s}=\{e_i\}$ and $\mathbf{s}'=\{e'_i\}$ are two seeds (not necessarily mutation adjacent) in the same mutation equivalent family of seeds and that $\sigma^*:N\rightarrow N$ is a lattice isomorphism preserving the skew-symmetric form $\{\cdot,\cdot\}$ and such that $\sigma^*(\mathbf{s}')=\mathbf{s}$. (Let us denote the induced map $M\rightarrow M$ also by $\sigma^*$.) Then these two dual maps induce the following isomorphisms between the respective seed tori
\begin{align*}
    \sigma: \mathcal{A}_\mathbf{s}&\longrightarrow \mathcal{A}_{\mathbf{s}'} & \sigma:\mathcal{X}_\mathbf{s}&\longrightarrow\mathcal{X}_{\mathbf{s}'}\\
    \sigma^*(A^m)&:=A^{\sigma^*(m)} & \sigma^*(X^n)&:=X^{\sigma^*(n)}. 
\end{align*}
Since $\sigma^*$ preserves the skew-symmetric form, $\sigma^*$ commutes with seed mutation as well, i.e., $\sigma^*(\mu_{e_k}\mathbf{s}')=\mu_{\sigma^*(e_k)}\mathbf{s}$. Thus, the above isomorphisms of algebraic tori also commute with the birational mutation maps and, as a result, we obtain a pair of automorphisms $\sigma:\mathcal{A}\rightarrow \mathcal{A}$ and $\sigma:\mathcal{X}\rightarrow \mathcal{X}$ between the quasi-cluster varieties. By definition, we refer to any such automorphisms of the quasi-cluster varieties as \emph{quasi-cluster transformations}.
